# Supplementary material for: A Benign Activity Extraction Method for Malignant Activity Identification using Data Provenance
Source: arXiv:2503.19370 source file (2025-03-25)
Supplement: Supplementary file 1 [file appendix3.tex]

\chapter{Code Examples}

For some projects, it might be relevant to include some code extracts in an appendix. You are not expected to put all of your code here - the correct place for all of your code is in the technical submission that is made in addition to the Final Report. However, if there are some notable aspects of the code that you discuss, including that in an appendix might be useful to make it easier for your readers to access. 

As a general guide, if you are discussing short extracts of code then you are advised to include such code in the body of the report. If there is a longer extract that is relevant, then you might include it as shown in the following section. 

Only include code in the appendix if that code is discussed and referred to in the body of the report. 

\section{Random Number Generator}

The Bayes Durham Shuffle ensures that the psuedo random numbers used in the simulation are further shuffled, ensuring minimal correlation between subsequent random outputs \cite{NumericalRecipes}.

\begin{verbatim}
 #define IM1 2147483563
 #define IM2 2147483399
 #define AM (1.0/IM1)
 #define IMM1 (IM1-1)
 #define IA1 40014
 #define IA2 40692 
 #define IQ1 53668
 #define IQ2 52774
 #define IR1 12211
 #define IR2 3791
 #define NTAB 32
 #define NDIV (1+IMM1/NTAB)
 #define EPS 1.2e-7
 #define RNMX (1.0 - EPS)
 
 double ran2(long *idum)
 {
   /*---------------------------------------------------*/
   /* Minimum Standard Random Number Generator          */
   /* Taken from Numerical recipies in C                */
   /* Based on Park and Miller with Bays Durham Shuffle */
   /* Coupled Schrage methods for extra periodicity     */
   /* Always call with negative number to initialise    */
   /*---------------------------------------------------*/	
 
   int j;
   long k;
   static long idum2=123456789;
   static long iy=0;
   static long iv[NTAB];
   double temp;
 
   if (*idum <=0)
   {
     if (-(*idum) < 1)
     {
       *idum = 1;
     }else
     {
       *idum = -(*idum);
     }
     idum2=(*idum);
     for (j=NTAB+7;j>=0;j--)
     {
       k = (*idum)/IQ1;
       *idum = IA1 *(*idum-k*IQ1) - IR1*k;
       if (*idum < 0)
       {
         *idum += IM1;
       }
       if (j < NTAB)
       {
         iv[j] = *idum;
       }
     }
     iy = iv[0];	
   }
   k = (*idum)/IQ1;
   *idum = IA1*(*idum-k*IQ1) - IR1*k;
   if (*idum < 0)
   {
     *idum += IM1;
   }
   k = (idum2)/IQ2;
   idum2 = IA2*(idum2-k*IQ2) - IR2*k;
   if (idum2 < 0)
   {
     idum2 += IM2;
   }
   j = iy/NDIV;
   iy=iv[j] - idum2;
   iv[j] = *idum;
   if (iy < 1)
   {
     iy += IMM1;
   }
   if ((temp=AM*iy) > RNMX)
   {
     return RNMX;
   }else
   {
     return temp;	
   }
 }
 
\end{verbatim}
