# Supplementary material for: A Benign Activity Extraction Method for Malignant Activity Identification using Data Provenance
Source: arXiv:2503.19370 source file (2025-03-25)
Supplement: Supplementary file 2 [file appendix1.tex]

\chapter{Third-Party Code and Libraries}

If you have made use of any third party code or software libraries, i.e. any code that you have not designed and written yourself, then you must include this appendix. 

As has been said in lectures, it is acceptable and likely that you will make use of third-party code and software libraries. If third party code or libraries are used, your work will build on that to produce notable new work. The key requirement is that we understand what is your original work and what work is based on that of other people. 

Therefore, you need to clearly state what you have used and where the original material can be found. Also, if you have made any changes to the original versions, you must explain what you have changed. 

As an example, you might include a definition such as: 

Apache POI library - The project has been used to read and write Microsoft Excel files (XLS) as part of the interaction with the client's existing system for processing data. Version 3.10-FINAL was used. The library is open source and it is available from the Apache Software Foundation 
\cite{apache_poi}. The library is released using the Apache License 
\cite{apache_license}. This library was used without modification.
