# Supplementary material for: A Benign Activity Extraction Method for Malignant Activity Identification using Data Provenance
Source: arXiv:2503.19370 source file (2025-03-25)
Supplement: Supplementary file 3 [file appendix2.tex]

\chapter{Ethics Submission}

This appendix includes a copy of the ethics submission for the project. After you have completed your Ethics submission, you will receive a PDF with a summary of the comments. That document should be embedded in this report, either as images, an embedded PDF or as copied text. The content should also include the Ethics Application Number that you receive.
